# Supplementary material for: TopoHR: Hierarchical Centerline Representation for Cyclic Topology Reasoning in Driving Scenes with Point-to-Instance Relations
Source: arXiv:2604.24119 source file (2026-06-10)
Supplement: Supplementary file 1 [file 6_appendix.tex]

% \clearpage
% \onecolumn

\clearpage
\setcounter{page}{1}
\appendix
\maketitlesupplementary

% \section{Supplementary Materials for TopoHR}
In this supplementary material, we provide additional analysis of the proposed TopoHR, including:
\begin{itemize}
\item Analysis of computational complexity.

\item More ablation studies on the OpenLane-V2 subset\_B split.

\item More point-to-instance topology prediction results.

\item Qualitative analysis on OpenLane-V2 dataset.

\item Future works.

% \item Source Code.
\end{itemize}

\section{Analysis of Computational Complexity}

Table~\ref{tab:params and fps} reports model size, inference speed, and accuracy on the OpenLane-V2 subset\_A validation set. TopoLogic~\cite{fu2024topologic} serves as the original baseline. To build a memory-efficient reference, we re-implement it without the GNN module while keeping the same topology reasoning design (“TopoHR, Ins”). This reduces parameters from 62.1MB to 54.9MB and slightly improves inference speed (24.4 → 25.2 FPS), forming a lighter baseline.
Building upon this baseline, introducing point-level representation (“Ins+Pts”) increases parameters only marginally (54.9MB → 59.7MB) while yielding clear accuracy gains. Further adding segmentation supervision (“Ins+Pts+Seg”) increases parameters by only 13.8\% (54.9MB → 62.5MB) but substantially improves both $\mathrm{DET}_{\text{l}}$ and $\mathrm{TOP}_{\text{ll}}$. Notably, even without cyclic enhancement, this variant already outperforms TopoLogic with comparable parameters (62.1MB vs. 62.5MB), highlighting the effectiveness of the hierarchical representation.
Enabling the cyclic pipeline and P2I relation further improves topology reasoning, achieving the best overall accuracy while maintaining competitive speed. For comparison, the second row increases the decoder depth of TopoLogic to match the parameter scale but yields only marginal gains, confirming that TopoHR’s improvements stem from hierarchical representation and cyclic reasoning rather than model size. Overall, each component demonstrate that each architectural enhancement offers favorable accuracy–efficiency trade-offs, with the segmentation-augmented representation offering particularly strong gains for its modest parameter increase.

\begin{table}[h]
    \centering
    \fontsize{9pt}{9pt}\selectfont
    \setlength{\tabcolsep}{1.5pt} % 减小列间空白（默认约6pt）
     % 减小行高（默认约1.2）
    \caption{Comparison with different methods on OpenLane-V2 subset\_A val set. FPSs are measured on one NVIDIA RTX 4090 GPU with batch size as 1. \#L: number of decoder layers.}
    \begin{tabular}{ccc|ccc|cc}
    \toprule 
         Method & Repr & Cyclic & \#L & Params & FPS & $\mathrm{DET}_{\text{l}}$ & $\mathrm{TOP}_{\text{ll}}$\\
         \midrule
         TopoLogic & Ins & - & 6 & 62.1MB & 24.4 & 29.9 & 23.9 \\
         TopoLogic* & Ins & - & 12 & 89.5MB & 10.8 & 30.2 & 24.8 \\
         \cmidrule{1-8}
         TopoHR & Ins & - & 6 & 54.9MB & 25.2 & 26.8 & 23.1\\
         TopoHR & Ins+Pts & - & 6 & 59.7MB & 23.0 & 32.2 & 26.3\\
         % \cmidrule{1-8}
         % TopoHR & Ins+Pts & - & 59.7MB & 23.0 & 32.2 & 26.3\\
         % \cmidrule{1-8}
         TopoHR & Ins+Pts+Seg & - & 6 & 62.5MB & 13.3 &34.6 & 30.6\\
         % \cmidrule{1-8}
         \cellcolor[HTML]{DADADA}TopoHR & \cellcolor[HTML]{DADADA}Ins+Pts+Seg & \cellcolor[HTML]{DADADA}\checkmark & \cellcolor[HTML]{DADADA}6 & \cellcolor[HTML]{DADADA}83.1MB & \cellcolor[HTML]{DADADA}12.6 & \cellcolor[HTML]{DADADA}36.1 & \cellcolor[HTML]{DADADA}31.8\\
    \bottomrule
    \end{tabular}
    \label{tab:params and fps}
\end{table}

\section{More Abltion Study}
We similarly validated the effectiveness of each TopoHR component in the split of subset\_B. The setup for the ablation study remains consistent with the Section~\ref{sec:ablation study}.

\vspace{.5mm}\noindent\textbf{Hierarchical Centerline Representation.}
Table~\ref{tab:ablation of Hierarchical Centerline Representation on subset_B} shows that adding point-level constraints and the hierarchical integrator already provides a clear improvement over the instance-only baseline, reaching 28.0 $\mathrm{DET}_{\text{l}}$ and 25.2 $\mathrm{TOP}_{\text{ll}}$. This confirms that aligning local geometric cues with global instance structure is essential. Incorporating segmentation supervision further boosts performance. Binary (0/1) masks raise the scores to 30.6 $\mathrm{DET}_{\text{l}}$ and 29.6 $\mathrm{TOP}_{\text{ll}}$, and Distance Transform (DT) masks offer additional gains. Our Discrete Distance Transform (DDT) mask performs best, improving the baseline by 5.9 $\mathrm{DET}_{\text{l}}$ and 9.1 $\mathrm{TOP}_{\text{ll}}$. Overall, each component of the hierarchical centerline representation contributes meaningfully, and the full design yields the strongest results.

\begin{table}[h]
    \centering
    % \fontsize{9pt}{9pt}\selectfont
    \fontsize{9pt}{9pt}\selectfont
    \setlength{\tabcolsep}{2pt} % 减小列间空白（默认约6pt）
     % 减小行高（默认约1.2）
    \caption{Ablation of hierarchical centerline representation on subset\_B split. (P2P Constrain: P2P constrained relation mask; DT: distance transform mask; DDT: discrete distance transform mask.)}
    \begin{tabular}{c|ccc|cccc}
    \toprule
         \multirow{2}{*}{Repr} & \multicolumn{1}{c}{P2P} & \multicolumn{1}{c}{Hierarchical} &   Seg &   \multirow{2}{*}{$\mathrm{DET}_{\text{l}}$} &  \multirow{2}{*}{$\mathrm{TOP}_{\text{ll}}$}  \\
         & Constrain & Integrator & GT & & \\
         \midrule
         Ins & - & - & - & 25.9 & 21.1\\
         % \addlinespace
         \cmidrule{1-6}
         % Ins+Pts  & - & - & - & &\\
         % Ins+Pts  & \checkmark & - & - &  & \\
         Ins+Pts  & \checkmark & \checkmark & - & 28.0 & 25.2\\
         % \addlinespace
         \cmidrule{1-6}
         Ins+Pts+Seg  & \checkmark & \checkmark & 0/1  &30.6 &29.6\\
         Ins+Pts+Seg  & \checkmark & \checkmark & DT &31.1 & 29.7\\
         \cellcolor[HTML]{DADADA}Ins+Pts+Seg & \cellcolor[HTML]{DADADA}\checkmark & \cellcolor[HTML]{DADADA}\checkmark & \cellcolor[HTML]{DADADA}DDT & \cellcolor[HTML]{DADADA}31.8 & \cellcolor[HTML]{DADADA}30.2\\
         \addlinespace
         \cmidrule{1-6}
         \hlg{\textit{Inprovement}} & - & - & - & \hlg{5.9$\uparrow$} & \hlg{9.1$\uparrow$}\\ 
    \bottomrule
    \end{tabular}
    \label{tab:ablation of Hierarchical Centerline Representation on subset_B}
\end{table}

\vspace{.5mm}\noindent\textbf{Cyclic Pipeline and P2I Relation.}
Table~\ref{tab:ablation of cyclic pipeline on subset_B} evaluates the cyclic information flow and hierarchical relation modeling under our hierarchical centerline representation and adaptive topological loss. Using only instance-level queries without cyclic feedback achieves 31.8 $\mathrm{DET}_{\text{l}}$ and 31.0 $\mathrm{TOP}_{\text{ll}}$. Introducing I2I attention in the forward path and feeding back I2I topological predictions improves $\mathrm{DET}_{\text{l}}$ and $\mathrm{TOP}_{\text{ll}}$ by 2.9 and 0.8, showing the benefit of iterative refinement. The full model which combines instance- and point-level queries with both I2I and P2I relations, achieves the best results, 35.3 $\mathrm{DET}_{\text{l}}$, 32.1 $\mathrm{TOP}_{\text{ll}}$, and 25.2 $\mathrm{TOP}_{\text{lt}}$. These findings confirm that cyclic modeling, especially the P2I relation, substantially strengthens both detection and topological reasoning. They further support our claim that topology emerges from complementary instance- and point-level representations.

\begin{table}[h]
    \centering
    \fontsize{9pt}{9pt}\selectfont
    \setlength{\tabcolsep}{2.5pt} % 减小列间空白（默认约6pt）
     % 减小行高（默认约1.2）
    \caption{Ablation of cyclic pipeline and P2I relation using hierarchical centerline representation and adaptive topological loss on subset\_B split.}
    \begin{tabular}{cc|c|ccc}
    \toprule
    % 第一行：为前6列设置标签，并为后2列预留标题位置
    \multicolumn{2}{c|}{Forward} & \multicolumn{1}{c|}{Backward} & \multirow{2}{*}{$\mathrm{DET}_{\text{l}}$} & \multirow{2}{*}{$\mathrm{TOP}_{\text{ll}}$} & \multirow{2}{*}{$\mathrm{TOP}_{\text{lt}}$} \\ 
    Query & Weight & Topo &  & &  \\
    % \addlinespace
    \midrule
    $\mathbf{Q}_{\text{ins}}$ & - & - & 31.8  & 31.0 & 22.8  \\
    \cmidrule{1-6}
    $\mathbf{Q}_{\text{ins}}$ & $\mathbf{W}_{\text{i2i}}$ & $\mathbf{T}_{\text{i2i}}$ & 34.7  & 31.8 & 23.5  \\
    % \addlinespace
    \cmidrule{1-6}
    % Ins+Pts & I2I & I2I & \cellcolor[HTML]{DADADA} & \cellcolor[HTML]{DADADA} \\
    \cellcolor[HTML]{DADADA}$\mathbf{Q}_{\text{ins}}$+$\mathbf{Q}_{\text{pts}}$ & \cellcolor[HTML]{DADADA}$\mathbf{W}_{\text{i2i}}$+$\mathbf{W}_{\text{p2i}}$ & \cellcolor[HTML]{DADADA}$\mathbf{T}_{\text{i2i}}$+$\mathbf{T}_{\text{p2i}}$ & \cellcolor[HTML]{DADADA}35.3 & \cellcolor[HTML]{DADADA}32.1 & \cellcolor[HTML]{DADADA}25.2\\
    % \addlinespace
    \cmidrule{1-6}
    \hlg{\textit{Inprovement}} & - & - & \hlg{3.5$\uparrow$} & \hlg{1.1$\uparrow$} & \hlg{2.4$\uparrow$}\\ 
    \bottomrule
    \end{tabular}
    \label{tab:ablation of cyclic pipeline on subset_B}
\end{table}

\section{More Point-to-Instance Topology Prediction Results}
Figure~\ref{fig:heatmap_2} provides additional qualitative examples demonstrating the effect of point-to-instance topology prediction. Compared with global instance-to-instance reasoning, the point-level formulation captures finer structural cues and yields more granular connectivity patterns. These observations further support our hierarchical topology formulation: topological relationships emerge not only between centerline instances but also through their underlying point-level representations.
\begin{figure*}[h]
	\centering
	\includegraphics[width=\linewidth]{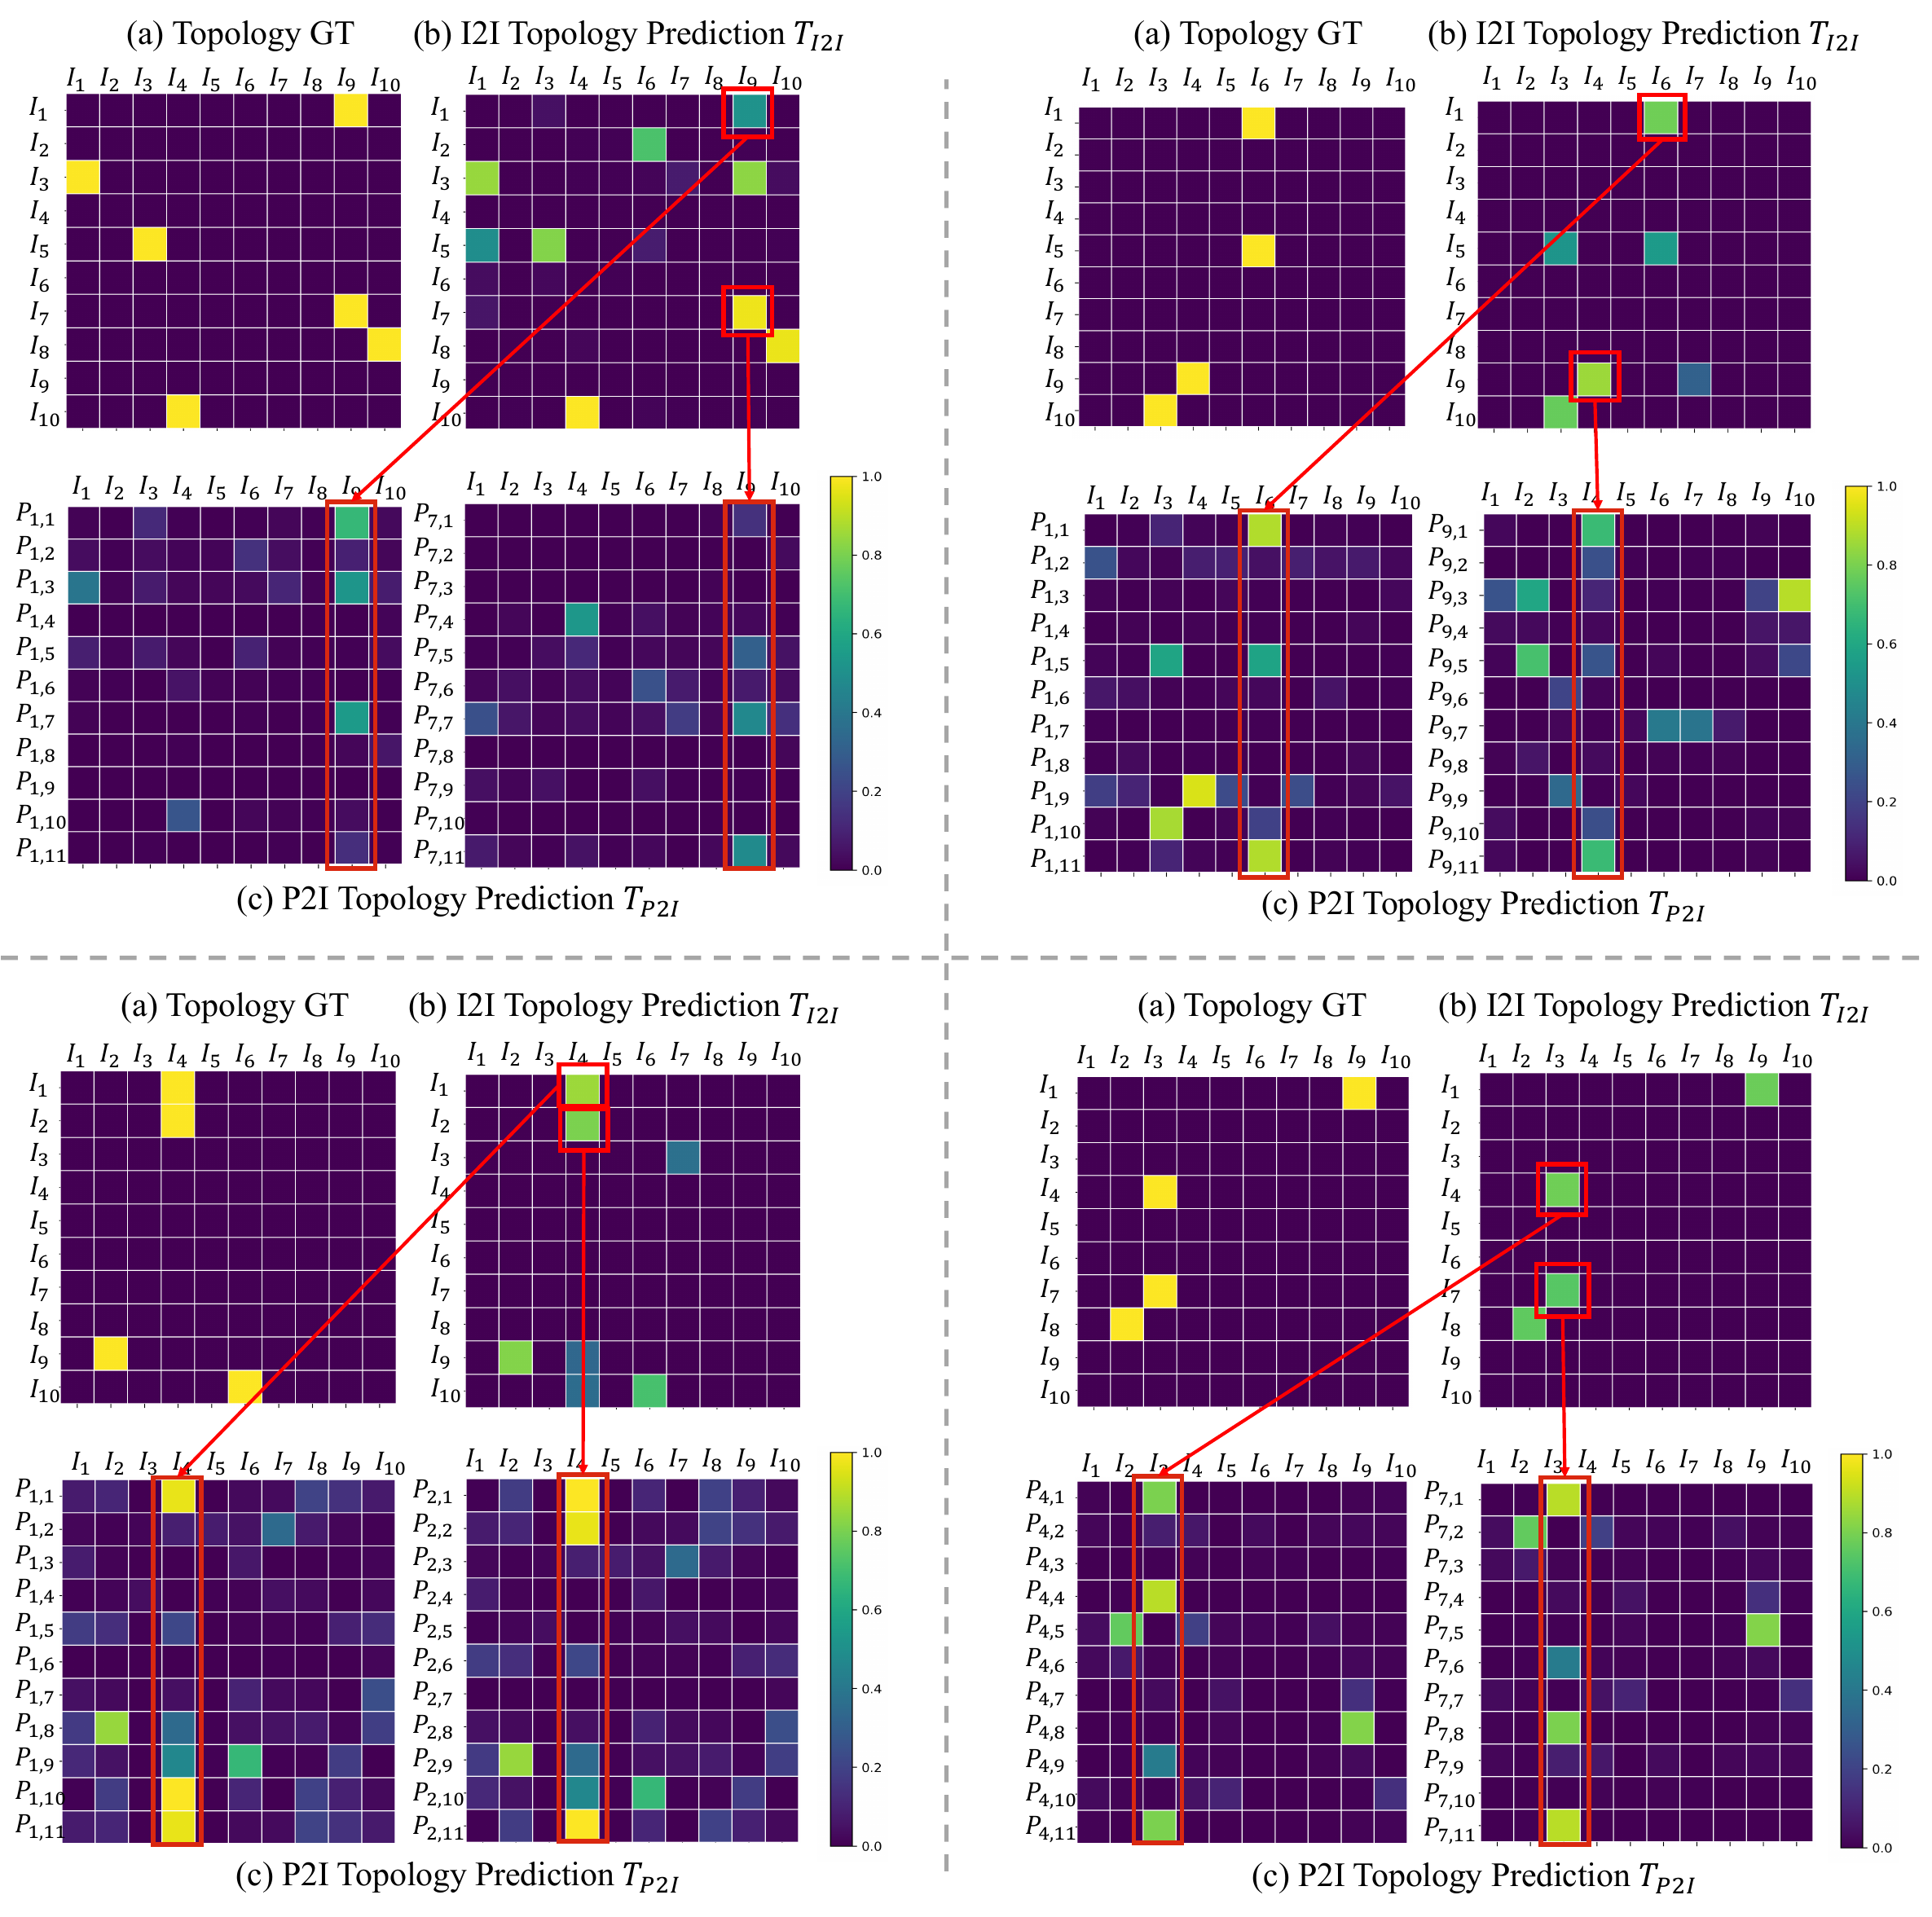}
	\caption{More instance-to-instance and point-to-instance topology reasoning results. (a) Groundtruth of centerline topology reasoning, where $(I_i, I_j) = 1$ denotes that the endpoint of the $I_i$-th centerline is connected to the start point of the $I_j$-th centerline. (b) Global instance-to-instance topology prediction. (c) Fine-grained point-to-instance topology prediction.}  
	\label{fig:heatmap_2}
\end{figure*}

\section{Qualitative Analysis}
We provide further qualitative results to illustrate the effectiveness of TopoHR in both detection and topological reasoning. Figures~\ref{fig:vis-1} and \ref{fig:vis-2} show diverse driving scenes from the OpenLane-V2 validation set. For each scene, the front-view image is shown on the left and the surround-view representation on the right. Detected centerlines are drawn as solid blue curves, while traffic elements are visualized as bounding boxes. Centerlines associated with traffic elements of a specific color are highlighted in the matching color to indicate predicted topological relations.
TopoHR consistently delivers strong performance across varied scenarios, producing accurate centerline and traffic-element detections alongside reliable topology reasoning for both centerline-to-centerline and centerline-to-traffic relations. These results demonstrate that the combination of our cyclic pipeline, hierarchical centerline representation, and point-to-instance relation modeling yields robust improvements in both geometric perception and structured reasoning.

\section{Limitations and Future Work}
Although our method demonstrates strong performance in centerline topology reasoning, building more robust and accurate associations between traffic elements and centerlines remains a challenging problem. These associations are often influenced by the complexity of the scene, occlusion, and the diverse geometric layouts encountered in real driving scenarios. Improving the stability and precision of such cross-entity reasoning will therefore be an important direction of our future work. To this end, we are exploring differentiable neural geometric interfaces that can better integrate structural and semantic cues, with the goal of further enhancing cross-modal reasoning capabilities.

% \section{Source Code}
% We provide the source code for reference at $./\text{TopoHR}$. All dependencies and environment setup instructions can be found in the official TopoLogic repository~\cite{fu2024topologic}. The complete TopoHR repository will be made publicly available upon acceptance.

\begin{figure*}[htbp]
    \centering
    \begin{subfigure}[c]{\textwidth}
        \centering
        \includegraphics[width=0.85\linewidth]{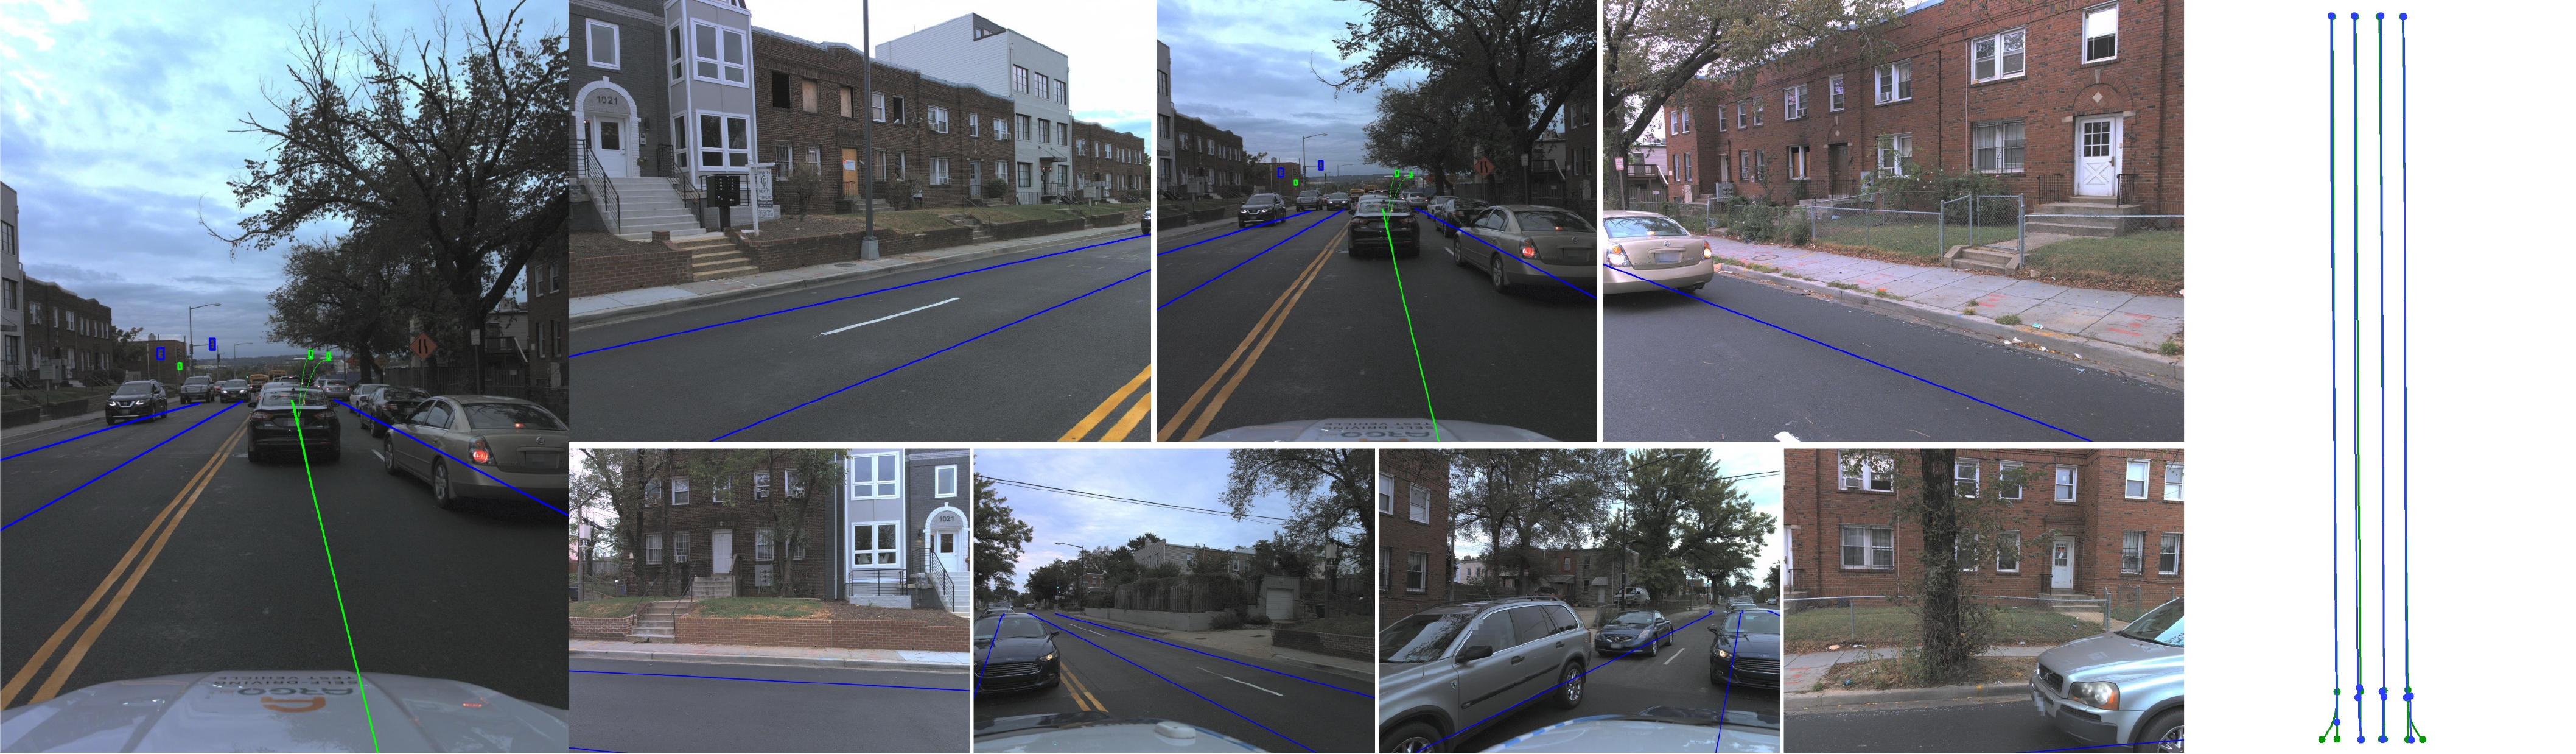}
    \end{subfigure}\\
    \medskip
    \begin{subfigure}[c]{\textwidth}
        \centering
        \includegraphics[width=0.85\linewidth]{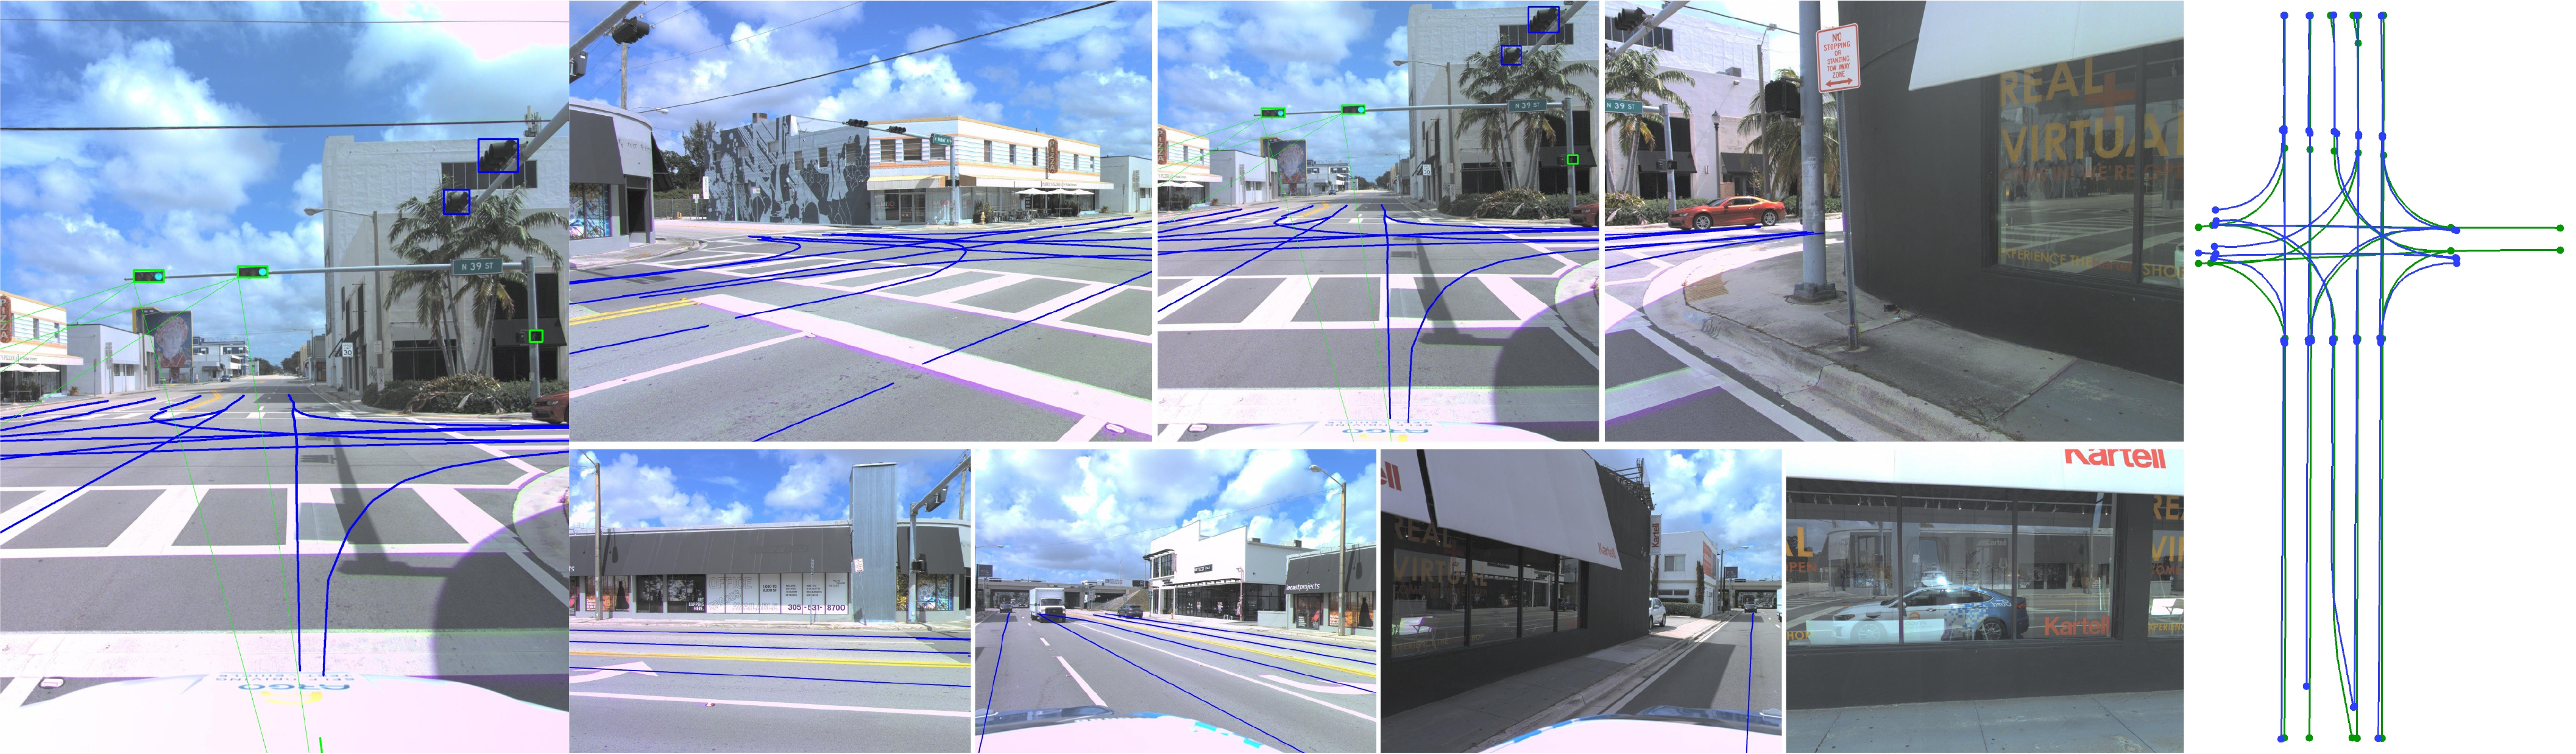}
    \end{subfigure}\\
    \medskip
    \begin{subfigure}[c]{\textwidth}
        \centering
        \includegraphics[width=0.85\linewidth]{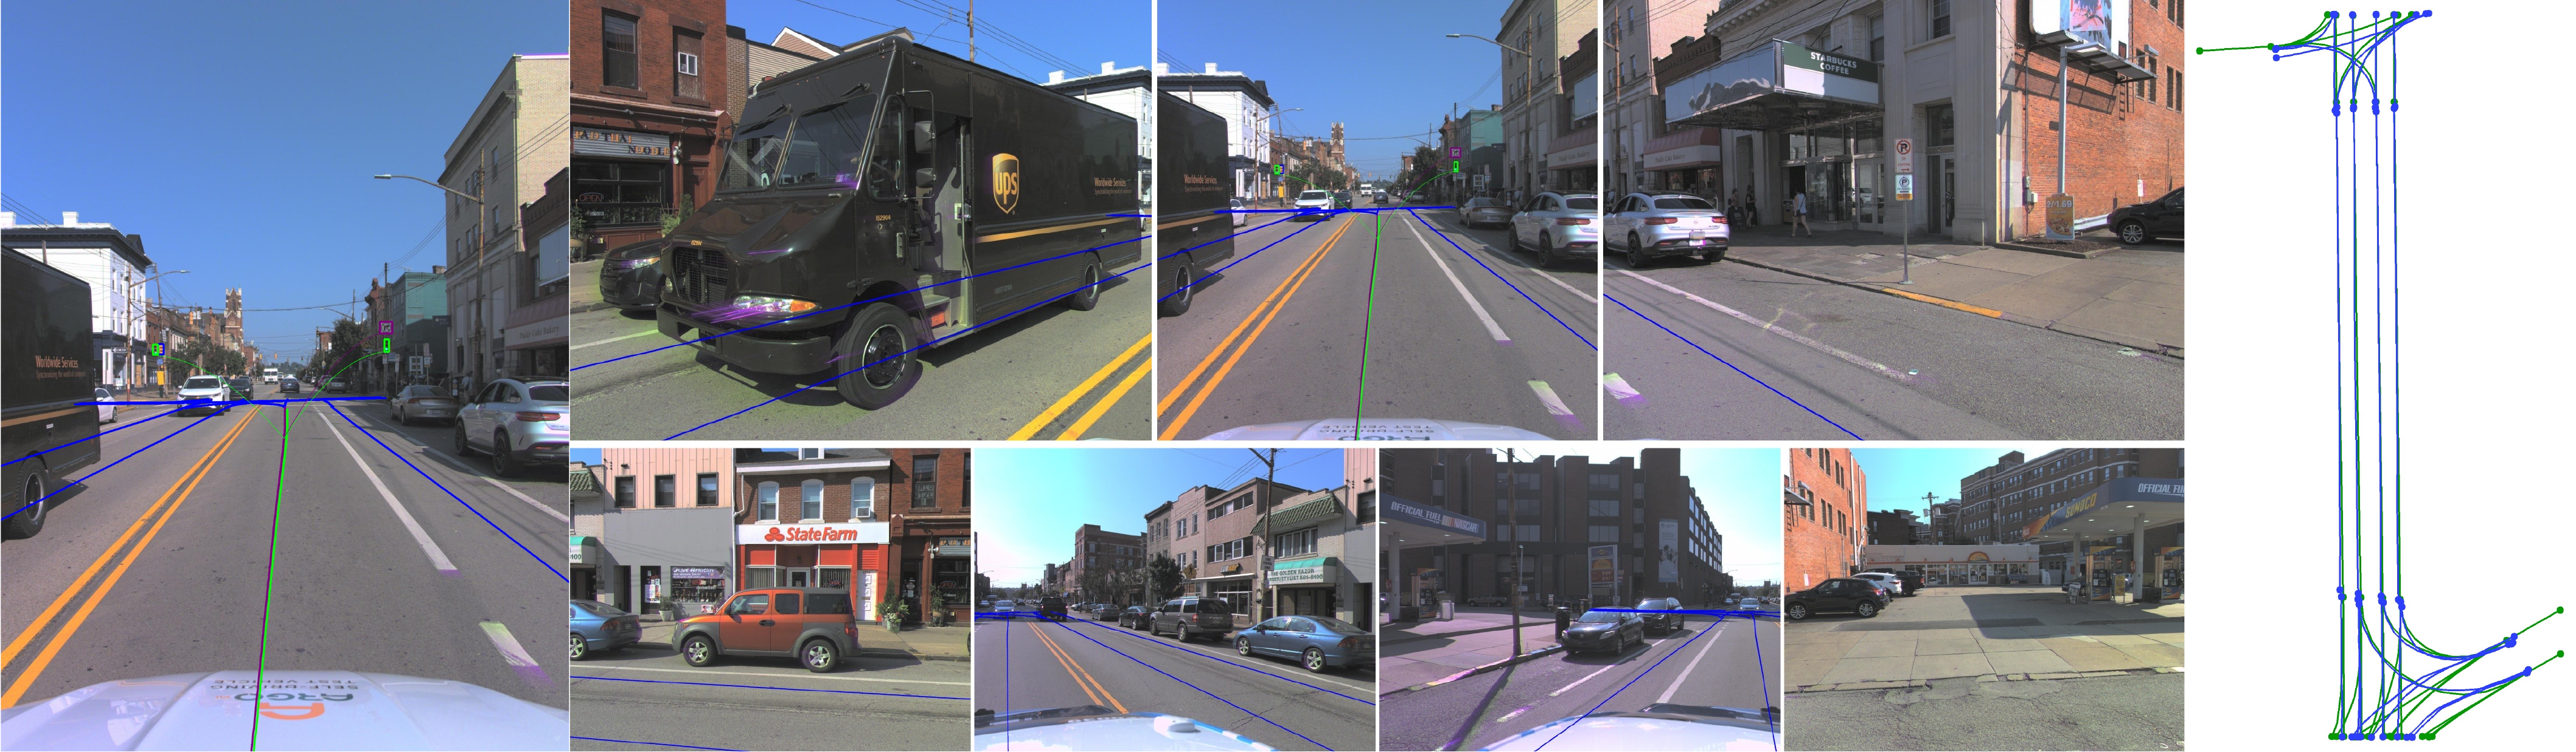}
    \end{subfigure}\\
    \medskip
    \begin{subfigure}[c]{\textwidth}
        \centering
        \includegraphics[width=0.85\linewidth]{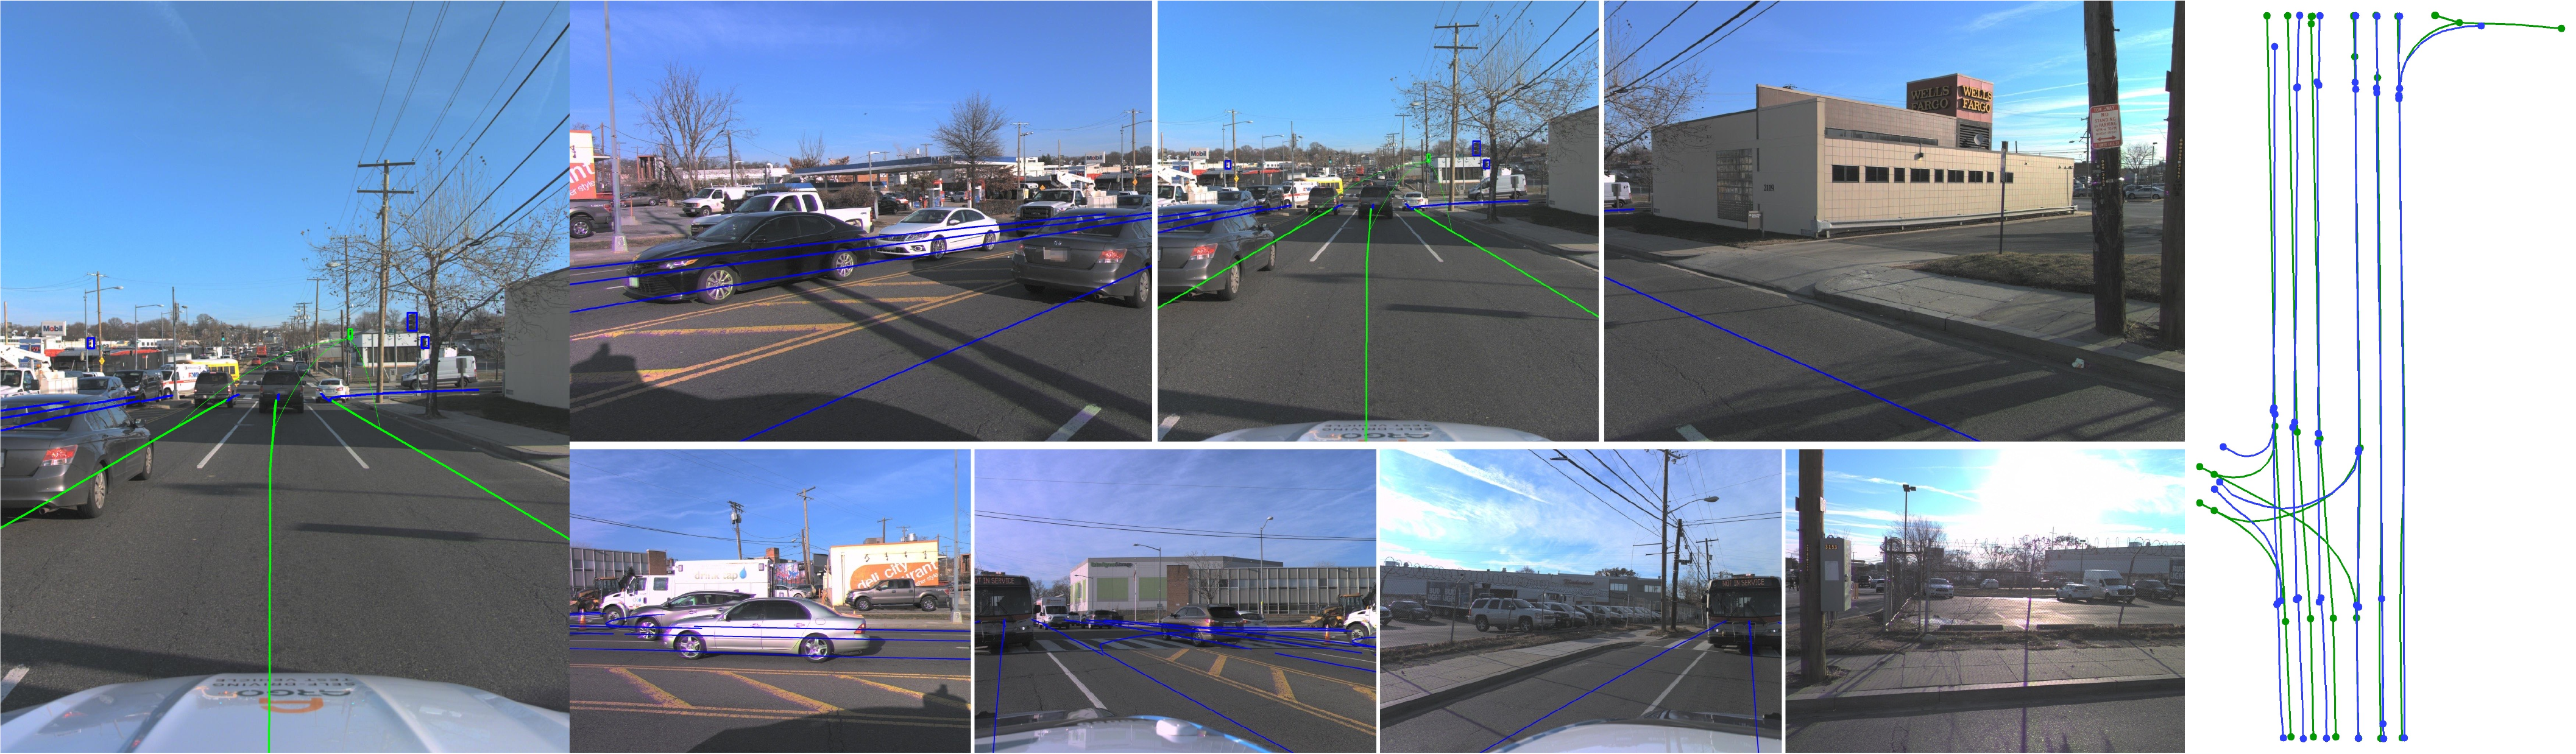}
    \end{subfigure}
    \caption{Illustration of detection and topology reasoning results on OpenLane-V2 validation dataset.}
    \label{fig:vis-1}
\end{figure*}

\begin{figure*}[htbp]
    \centering
    \begin{subfigure}[c]{\textwidth}
        \centering
        \includegraphics[width=0.85\linewidth]{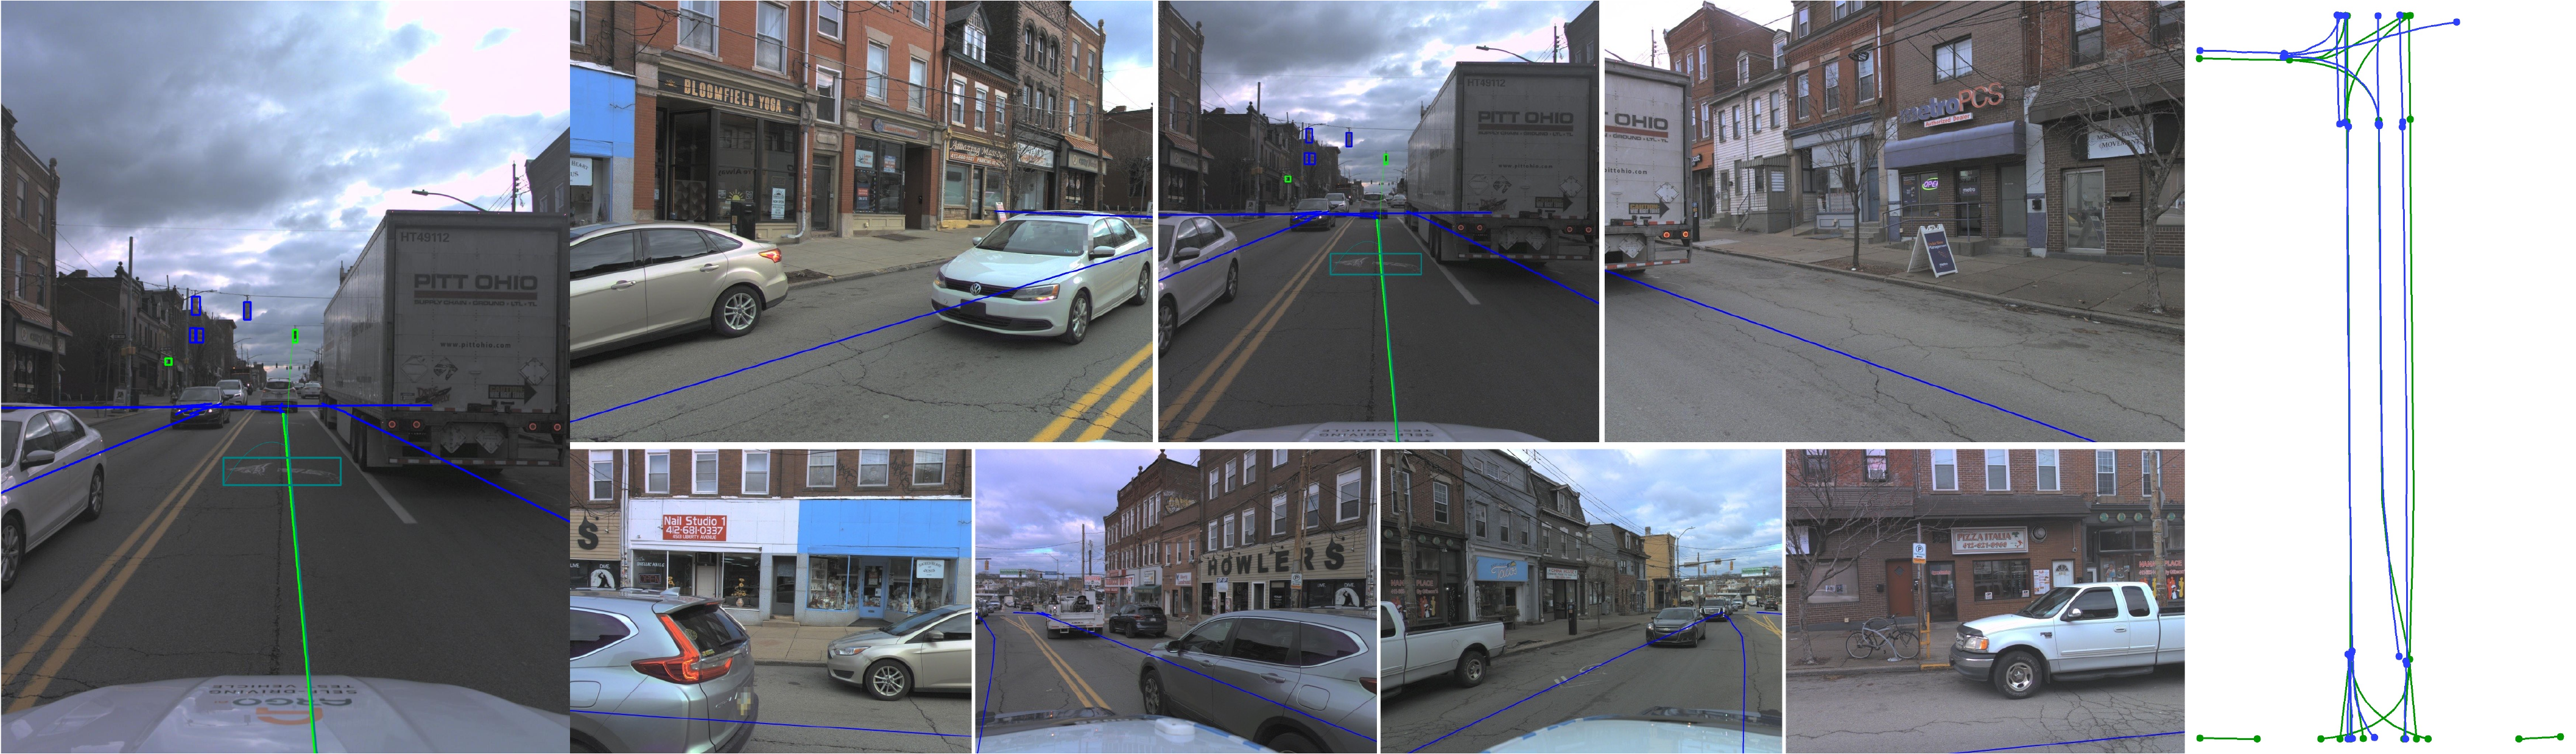}
    \end{subfigure}\\
    \medskip
    \begin{subfigure}[c]{\textwidth}
        \centering
        \includegraphics[width=0.85\linewidth]{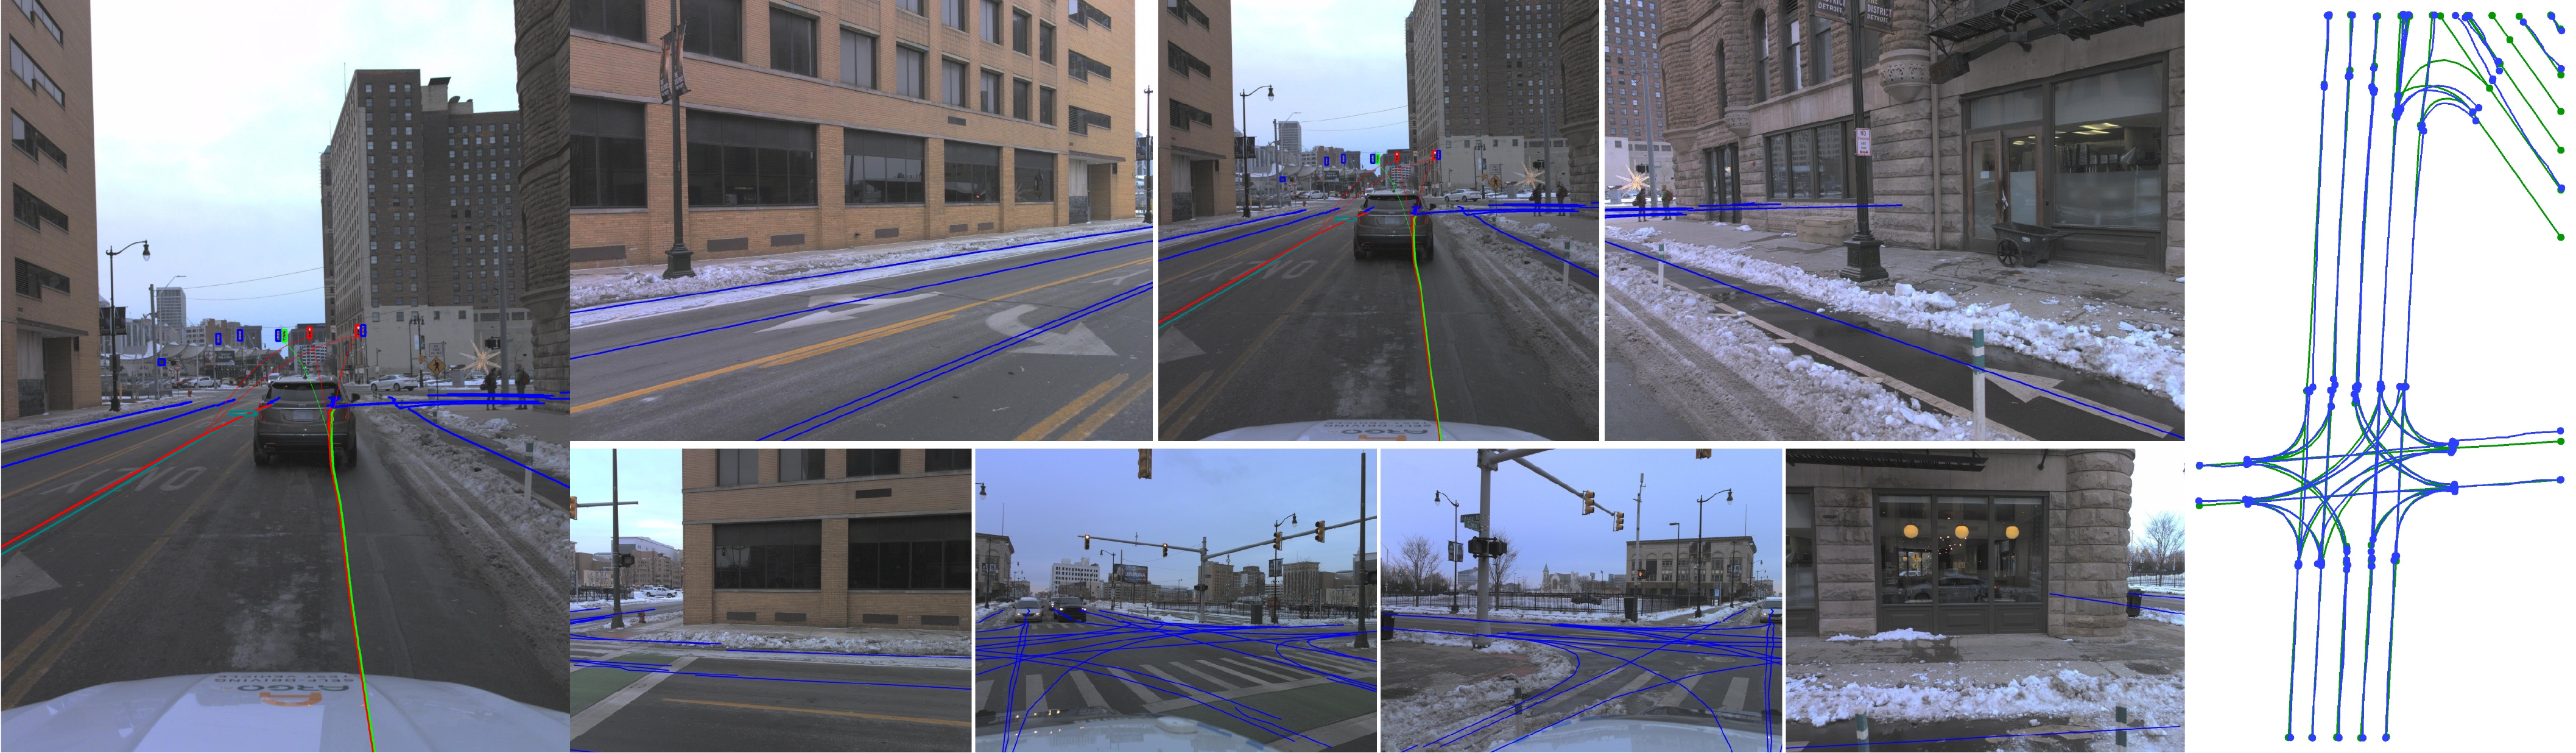}
    \end{subfigure}\\
    \medskip
    \begin{subfigure}[c]{\textwidth}
        \centering
        \includegraphics[width=0.85\linewidth]{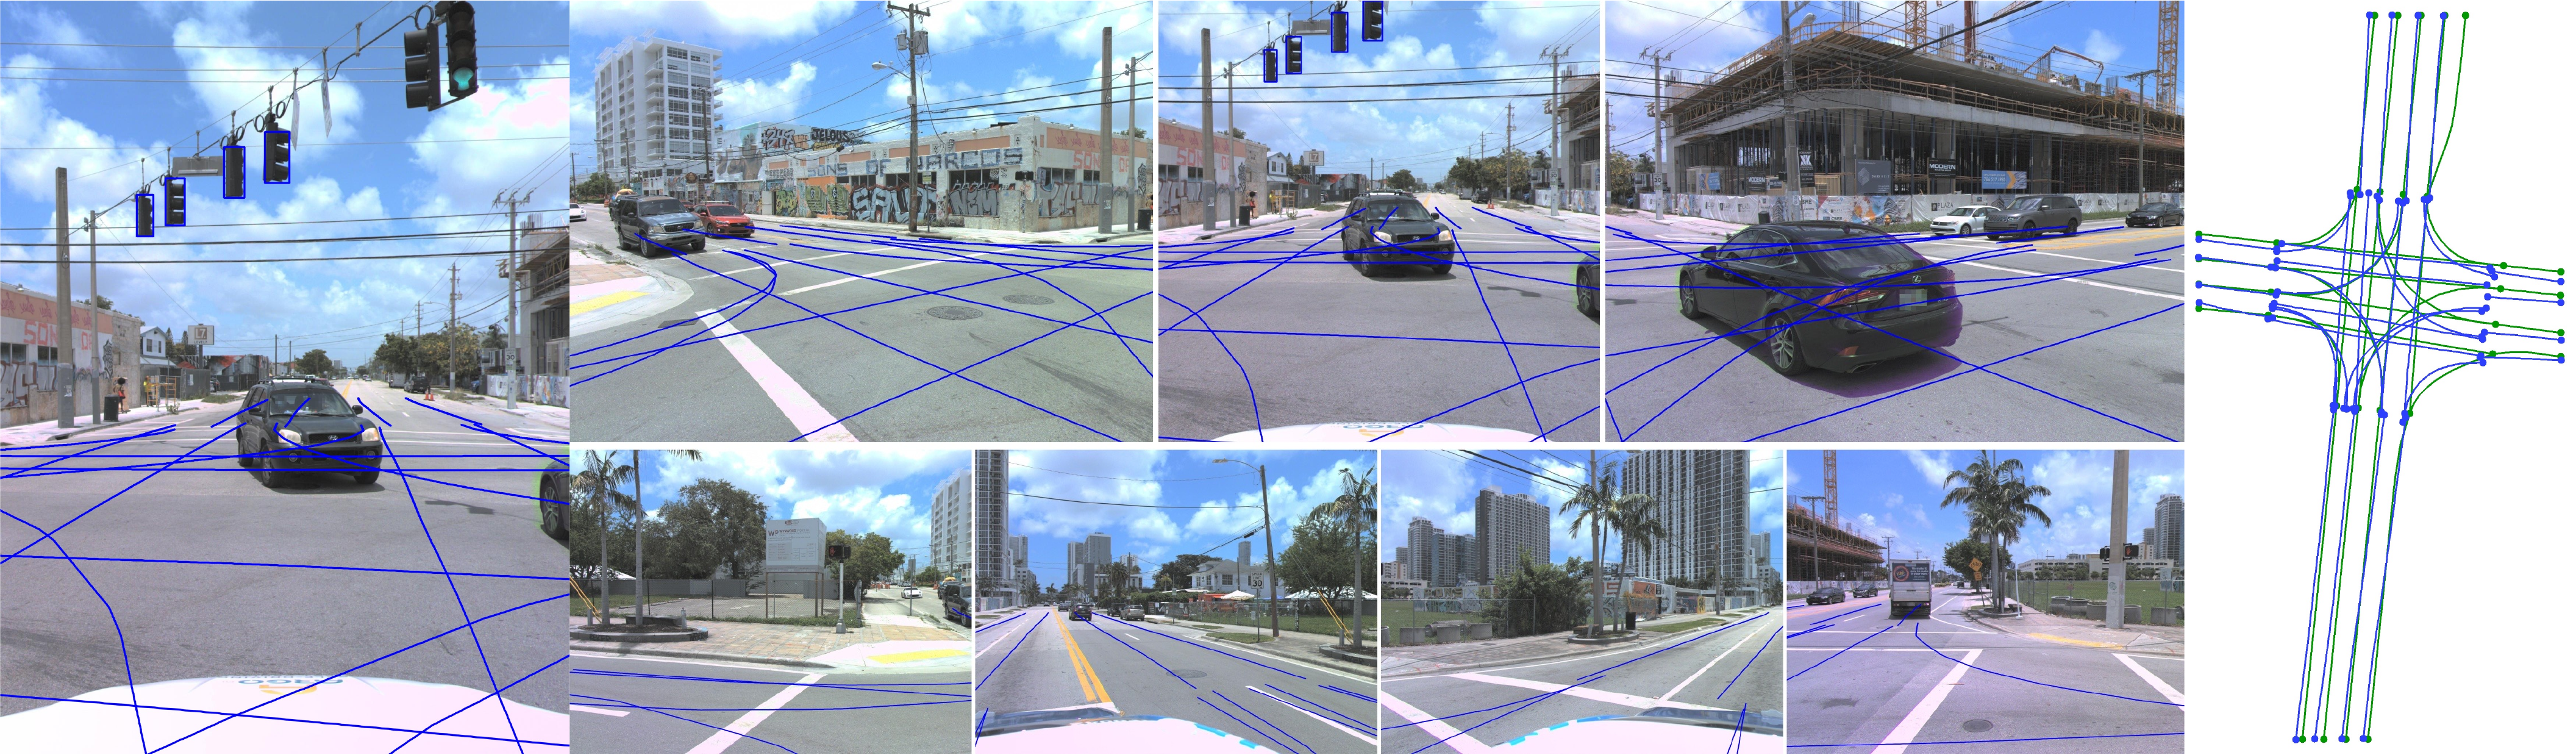}
    \end{subfigure}\\
    \medskip
    \begin{subfigure}[c]{\textwidth}
        \centering
        \includegraphics[width=0.85\linewidth]{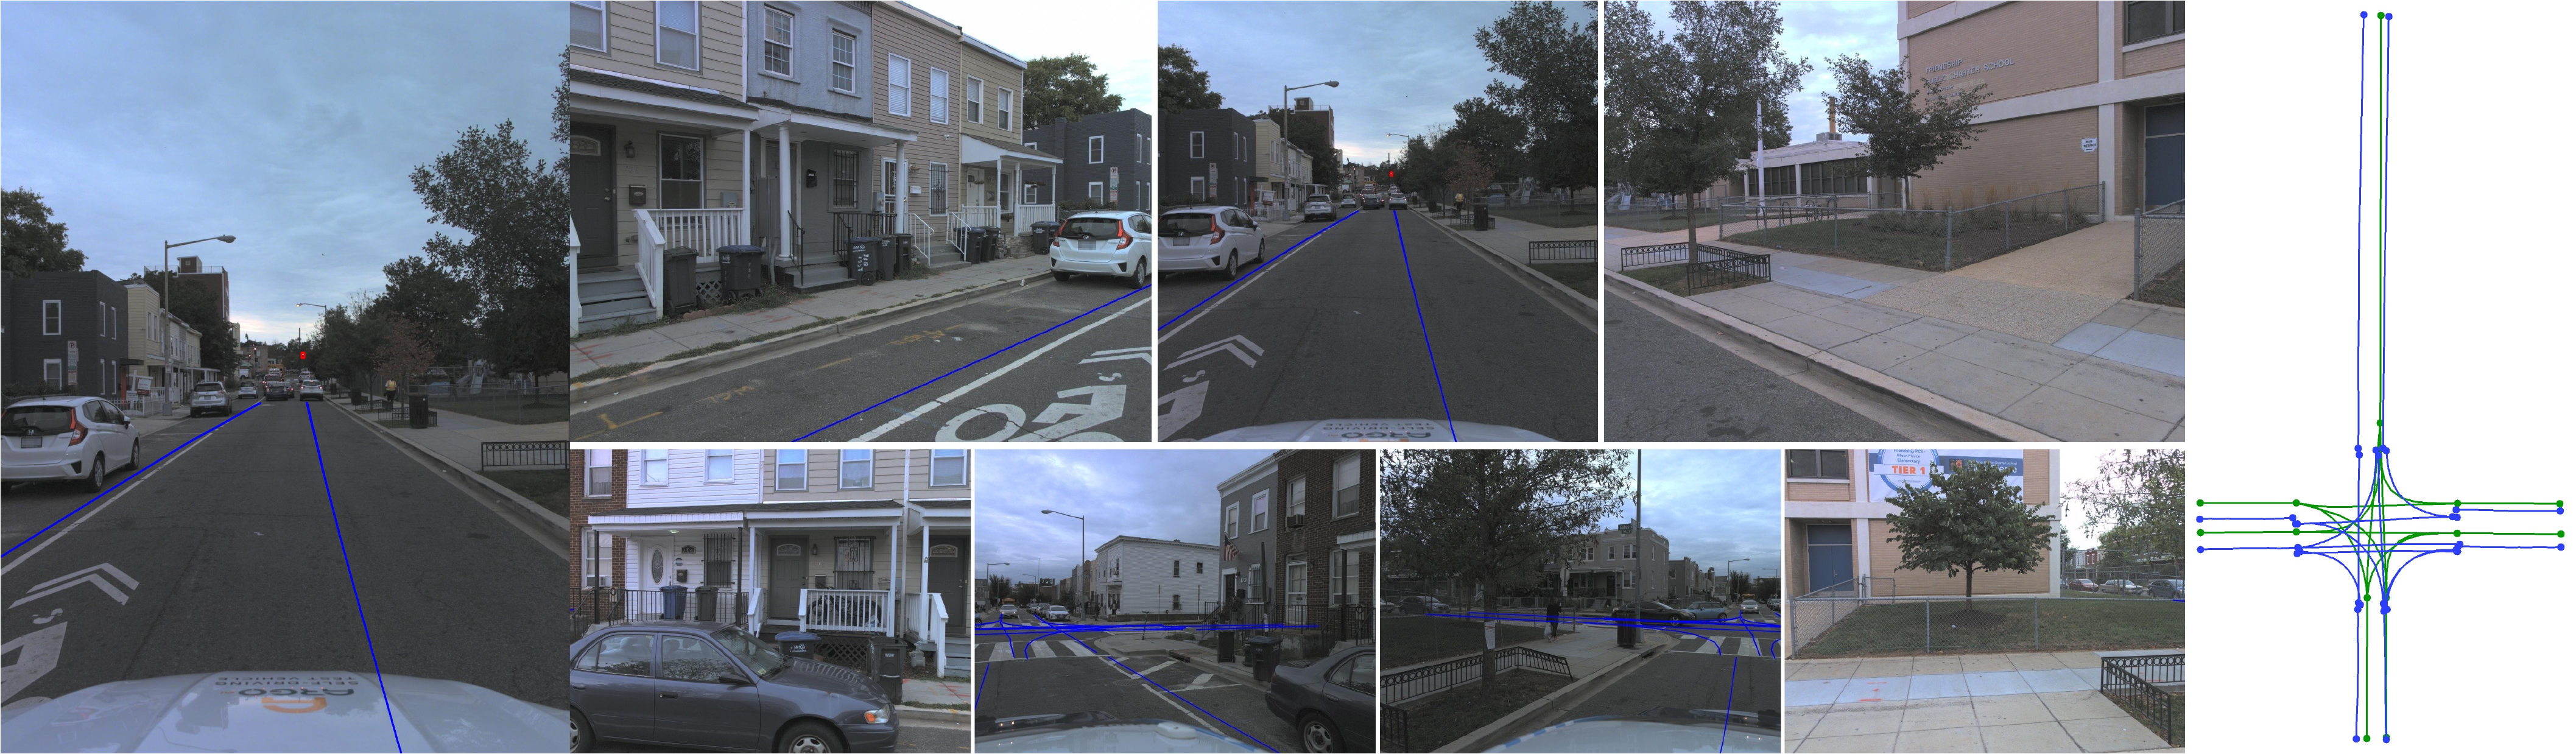}
    \end{subfigure}
    \caption{More qualitative results. With our proposed designs, TopoHR achieves more accurate reasoning of both centerline-to-centerline and centerline-to-traffic topological relationships.}
    \label{fig:vis-2}
\end{figure*}
